# Supplementary material for: Optical phonons coupled to a Kitaev spin liquid
Source: arXiv:2103.09828 ancillary file (2021-03-17)
Supplement: Supplementary file 1 [file kophsup.pdf]

# Supplemental Material for: Optical phonons coupled to a Kitaev spin liquid


A. Metavitsiadis,[1,*] W. Natori,[2,3,†] J. Knolle,[4,5,2,‡] and W. Brenig[1,§]

[1] Institute for Theoretical Physics, Technical University Braunschweig, D-38106 Braunschweig, Germany
[2] Blackett Laboratory, Imperial College London, London SW7 2AZ, United Kingdom
[3] Institut Laue-Langevin, BP 156, 41 Avenue des Martyrs, 38042 Grenoble Cedex 9, France
[4] Department of Physics TQM, Technical University of Munich, 85748 Garching, Germany
[5] Munich Center for Quantum Science and Technology (MCQST), Schellingstrasse 4, D-80799 München, Germany



In this Supplemental Material, we compile additional results and technical details. In Sec. I, we present microscopic justifications leading to Eq. (2) of the manuscript. In Sec. II, we extent our results to include a magnetic field, weak enough to be accessible perturbatively in the fermionic representation. Moreover, we detail the complete momentum dependence of the self-energy. In Sec. III, we describe the numerical procedure to obtain results in the radom gauge state. Finally, in Sec. IV, we provide justifications for the phenomenological treatment of the Raman response, including scattering from phonons and Majorana fermions, leading to the Fano effect, described by Eq. (6) of the main text.


## I. EFFECT OF DISTORTIONS ON THE EFFECTIVE MODEL FOR KITAEV MATERIALS

The existence of two charge transfer paths that form perfect 90° angles is crucial for the implementation of the Kitaev materials in heavy-ion Mott insulators [S1]. We rederive the effective models as performed in Refs. [S1, S2] by including a path dependence on the hopping integral, which can be induced by asymmetric distortions of the octahedra. Let us first establish this section's notation. The underlying multi-orbital Hubbard model for Kitaev materials is $H_{\rm Hub} = \hat{V} + \hat{T}$ where $\hat{V}$ gives the onsite interactions among $t_{2g}$ holes that depend upon the Coulomb repulsion $U$ and the Hund's coupling $J_H$ [S3, S4]. The hopping term is the sum of three tight-binding models. Focusing at this point on two sites $i$ and $j$ located on a plane $xy$, they are written like [S2]

$$\begin{aligned}
\hat{T}_2^{(l)} &= -\sum_\sigma \left( t_{2,l} d^\dagger_{i,yz,\sigma} d_{j,zx,\sigma} + t^*_{2,l} d^\dagger_{j,zx,\sigma} d_{i,yz,\sigma} \right), \\
\hat{T}_2^{(u)} &= -\sum_\sigma \left( t_{2,u} d^\dagger_{i,zx,\sigma} d_{j,yz,\sigma} + t^*_{2,u} d^\dagger_{j,yz,\sigma} d_{i,zx,\sigma} \right), \\
\hat{T}_3 &= -t_3 \sum_\sigma \left( d^\dagger_{i,xy,\sigma} d_{j,xy,\sigma} + d^\dagger_{j,xy,\sigma} d_{i,xy,\sigma} \right), \\
\hat{T}_1 &= -t_1 \sum_\sigma \left( d^\dagger_{i,yz,\sigma} d_{j,yz,\sigma} + d^\dagger_{i,zx,\sigma} d_{j,zx,\sigma} + \text{h.c.} \right).
\end{aligned} \tag{S1}$$

The hopping terms $t_1$ and $t_3$ are mainly related to the direct overlap of the orbitals [S5] and, thus, we do not consider their dependence with the asymmetry of the two paths. However, $\hat{T}_2^{(u)}$ and $\hat{T}_2^{(l)}$ depends upon the superexchange routes and we distinguish the hopping integrals $t_{2,l}$ and $t_{2,u}$. For later reference, we write

$$t_{2,a} = t_2 + \delta t_{2,a}, \tag{S2}$$

where $t_2$ is the hopping integral in the idealized geometry with $\theta = 90°$ and $\delta t_{2,a}$ is the variation of the hopping as a function of the lattice distortion. In order to keep the greatest generality, we keep the possibility that $\delta t_{2,a}$ is complex, as it happens when an external magnetic field is applied [S6].

The effective model is obtained using standard second-order perturbation theory and is written like

$$\begin{aligned}
H_{ij}^{(z)} &= J \mathbf{S}_i \cdot \mathbf{S}_j + K S_i^z S_j^z + \Gamma \left( S_i^x S_j^y + S_i^y S_j^x \right) \\
&\quad + D \left( S_i^x S_j^y - S_i^y S_j^x \right) + h \left( s_i^z + s_j^z \right),
\end{aligned} \tag{S3}$$

where all coupling constants $\tilde{J}$ are given as a function of the direct Coulomb interaction $U$, the Hund's coupling $J_H$ and the hopping integrals $t_a$. For clarity, let us define the constants $\nu_1 = (3r_1 + r_2 + 2r_3)/6$ and $\nu_2 = (r_1 - r_2)/4$,

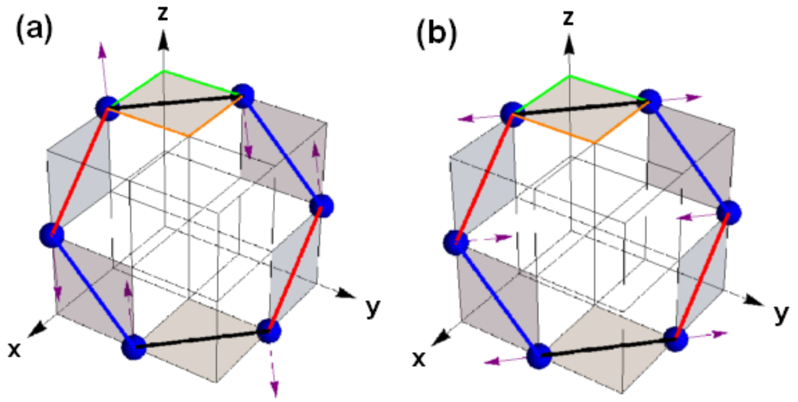


FIG. S1. Illustration of a Kitaev hexagon with the optical mode $E_{g2}$ indicated by purple arrows. The path assigned in orange (green) is called $l$ ($u$).

where $r_1 = U/(U-3J_H)$, $r_2 = U/(U-J_H)$ and $r_1 = U/(U+2J_H)$. The exact values of the coupling constants and the artificial magnetic field are

$$J = \frac{4}{9U}\left[\nu_1\left(4t_1^2 - (\mathrm{Im}t_{l,u})^2 - (\mathrm{Re}t_{l,u})^2\right) + 4(\nu_1+2\nu_2)t_1t_3 + (\nu_1-2\nu_2)t_3^2\right], \tag{S4a}$$

$$K = \frac{8}{9U}\left[2\nu_2(t_1-t_3)^2 + (\nu_1-\nu_2)|t|^2 - 2(\nu_1+2\nu_2)\mathbf{t}_l\cdot\mathbf{t}_u\right], \tag{S4b}$$

$$D = \frac{8}{9U}\mathrm{Re}t_{l,u}\left(2\nu_1t_1 + (\nu_1+2\nu_2)t_3\right), \tag{S4c}$$

$$\Gamma = \frac{16}{9U}\nu_2(t_1-t_3)\,\mathrm{Re}\left(t_{2,l}+t_{2,u}\right), \tag{S4d}$$

$$h = \frac{2}{9U}(r_1+r_2)(t_1-t_3)\,\mathrm{Im}t_{l,u}, \tag{S4e}$$

in which $t_{l,u} \equiv t_{2,l} - t_{2,u}$, $|t|^2 \equiv |t_{2,l}|^2 + |t_{2,u}|^2$ and $\mathbf{t}_l\cdot\mathbf{t}_u \equiv \mathrm{Re}t_{2,l}\mathrm{Re}t_{2,u} + \mathrm{Im}t_{2,l}\mathrm{Im}t_{2,u}$. The result in Eq. (S4) generalizes the results reported in Ref. [S6] by breaking the local inversion symmetry that induces a Dzyaloshinskii-Moriya interaction $D$ as a consequence. The exchange constants along $x$ and $y$ bonds have the same form, but the values of the hopping integrals should differ in a deformed system.

Let us now apply Eq. (S4) to the physically interesting case $t_1 = t_3 = 0$ and $t_{2,a}$ is real

$$J = -\frac{4}{9U}\nu_1\left(\delta t_{2,l} - \delta t_{2,u}\right)^2, \quad K = K_0\left(1 + \frac{\delta t_{2,l}+\delta t_{2,u}}{t_2}\right) + \mathcal{O}(\delta t_2^2), \tag{S5}$$

in which $K_0 = -\frac{16}{3U}\nu_2 t_2^2$ is the Kitaev coupling in the idealized geometry [S1, S2]. The Heisenberg coupling is set to zero when $t_2$ is identical in the two charge transfer paths, and is of order $\mathcal{O}(\delta t_2^2)$ otherwise. The second equation provides the microscopic justification to focus on the magnetoelastic coupling when $\delta t_{2,l} = \delta t_{2,u}$, which is expected to be true for usual distortions such as compression or elongation. In this case

$$\nabla K = \frac{2K_0}{t_2}\nabla t_2. \tag{S6}$$

## II. MAJORANA-PHONON COUPLING WITH FINITE MAGNETIC FIELD

A magnetic field can be included in the Kitaev spin Hamiltonian according to

$$H_K = \sum_{\mathbf{r}} \sum_{\boldsymbol{\delta}} J_{\boldsymbol{\delta}} S_{\mathbf{r}}^{d_{\boldsymbol{\delta}}} S_{\mathbf{r}-\boldsymbol{\delta}}^{d_{\boldsymbol{\delta}}} + g\mu_B \mathbf{B} \cdot \sum_{\mathbf{r}} \mathbf{S}_{\mathbf{r}} \ . \tag{S7}$$

We repeat here the notation conventions, $\mathbf{r} = l_1\mathbf{a}_1 + l_2\mathbf{a}_2$ runs over one sublattice, with $l_j = 0, 1, \dots, L-1$, for $j = 1, 2$, while $\boldsymbol{\delta}$ over the three vectors connecting the two sublattices. The vectors $\boldsymbol{\delta}$ and $\mathbf{a}$ are given by

$$\begin{bmatrix} \boldsymbol{\delta}_1 \\ \boldsymbol{\delta}_2 \\ \boldsymbol{\delta}_3 \end{bmatrix} = \frac{a}{2} \begin{bmatrix} \sqrt{3} & 1 \\ -\sqrt{3} & 1 \\ 0 & -2 \end{bmatrix} \begin{bmatrix} \boldsymbol{e}_x \\ \boldsymbol{e}_y \end{bmatrix} \quad \text{and} \quad \begin{bmatrix} \mathbf{a}_1 \\ \mathbf{a}_2 \\ \mathbf{a}_3 \end{bmatrix} = \frac{a\sqrt{3}}{2} \begin{bmatrix} 2 & 0 \\ 1 & \sqrt{3} \\ -1 & \sqrt{3} \end{bmatrix} \begin{bmatrix} \boldsymbol{e}_x \\ \boldsymbol{e}_y \end{bmatrix} \ . \tag{S8}$$

Furthermore, the indices $d_{\boldsymbol{\delta}}$ of the spin-1/2 operators $S$ acquire the values $d_{\boldsymbol{\delta}} = x, y, z$ depending on the $\boldsymbol{\delta}$-vector of the bond, while the Kitaev interactions $J_{\boldsymbol{\delta}}$, are considered isotropic. The magnetic field is $\mathbf{B} = (B, B, B)$, while $g = 1$ is the $g$-factor, $\mu_B = 1$ the Bohr magneton and we also set to unity the Planck and Boltzmann constants $\hbar, k_B = 1$.

Treating the magnetic field perturbatively for $B < \Delta$ enables a rewriting of Hamiltonian (S7) in terms of the Majorana fermions $c$ and $\bar{c}$ discussed in the main text [S7, S8]. In the fermionic representation, the Zeeman term of Eq. (S7) results in a next nearest neighbor (NNN) hopping. Therefore, regarding the spin subsystem, the Hamiltonian $H_K$ reads

$$H_K = H_1 + H_2 \ , \qquad \text{where,} \tag{S9}$$

$$H_1 = \sum_{\mathbf{r},\boldsymbol{\delta}} J_{\boldsymbol{\delta}} h_{\boldsymbol{\delta}}(\mathbf{r}) \ , \quad h_{\boldsymbol{\delta}}(\mathbf{r}) = -\frac{i}{4}\eta_{\boldsymbol{\delta}}(\mathbf{r}) c_{\mathbf{r}} c'_{\mathbf{r}-\boldsymbol{\delta}}$$

$$H_2 = -i\frac{\tilde{J}}{8} \sum_{\mathbf{r},\mathbf{a}} \left[ \zeta_{\mathbf{a}}(\mathbf{r}) c_{\mathbf{r}} c_{\mathbf{r}-\mathbf{a}} + \zeta'_{\mathbf{a}}(\mathbf{r}) c'_{\mathbf{r}-\boldsymbol{\delta}_3} c'_{\mathbf{r}-\boldsymbol{\delta}_3+\mathbf{a}} \right] .$$

$H_1$ is identical to that in Eq. (1) of the manuscript, with $\eta_{\boldsymbol{\delta}_1}(\mathbf{r}) = \eta_{\boldsymbol{\delta}_2}(\mathbf{r}) = 1$, and $\eta_{\boldsymbol{\delta}_3}(\mathbf{r}) = \pm 1$ corresponding to the $\mathbb{Z}_2$ gauge field arising from the freezing of the $\bar{c}$-species of the Majorana fermions. The prime on the second Majorana operator is introduced to discriminate between the two sublattices. $H_2$ follows from the fermionization of a three spin term which arises within third order perturbation theory from the spin model. The summation on $\mathbf{a}$ runs over the set of *three* $\mathbf{a}$ vectors described in Eq. (S8). The quantities $\zeta$ are given by

$$\zeta_{\mathbf{a}_1}(\mathbf{r}) = 1 \ , \quad \zeta_{\mathbf{a}_2}(\mathbf{r}) = -\eta_{\boldsymbol{\delta}_3}(\mathbf{r}) \ , \quad \zeta_{\mathbf{a}_3}(\mathbf{r}) = \eta_{\boldsymbol{\delta}_3}(\mathbf{r} - \mathbf{a}_1), \tag{S10a}$$

$$\zeta'_{\mathbf{a}_1}(\mathbf{r}) = 1 \ , \quad \zeta'_{\mathbf{a}_2}(\mathbf{r}) = -\eta_{\boldsymbol{\delta}_3}(\mathbf{r} - \mathbf{a}_1) \ , \quad \zeta'_{\mathbf{a}_3}(\mathbf{r}) = \eta_{\boldsymbol{\delta}_3}(\mathbf{r}) \ . \tag{S10b}$$

$\tilde{J}$ refers to the NNN effective three-spin coupling generated by the third order perturbation theory, $\tilde{J} \sim \frac{B^3}{\Delta^2}$, [S7, S8]. In order to stay in the perturbative regime, $B \lesssim B^* \approx \Delta$, meaning $\tilde{J} \sim O(10^{-2}J)$. It is important to realize, that although $\tilde{J}/J$ is only of the order of 1%, for real materials this corresponds to relatively strong magnetic fields of up to $B^* \approx 10T$. As we will see here, weak values of the effective NNN coupling term do not affect the high-frequency spectrum where the optical phonon modes lie.

Within the magnetoelastic scheme presented in the main text, the coupling of the two subsystems remains set by Eq. (2), i.e.

$$H_{KP} = \sum_{m\mathbf{q}} \mathcal{B}_{m\mathbf{q}} \mathcal{H}_{m,-\mathbf{q}} \ , \quad \mathcal{H}_{m\mathbf{q}} = \sum_{\boldsymbol{\delta}} \Lambda^{\boldsymbol{\delta}}_{m\mathbf{q}} h_{\boldsymbol{\delta};\mathbf{q}}, \tag{S11}$$

where $h_{\boldsymbol{\delta};\mathbf{q}}$ still refers *only* to the NN density, $\mathcal{B}_{m\mathbf{q}} = b_{m\mathbf{q}} + b^\dagger_{m,-\mathbf{q}}$ to the sum of phonon annihilation and creation operators at momentum $\pm\mathbf{q}$ and for polarization mode $m$, and the finite-momentum couplings are

$$\Lambda^{\boldsymbol{\delta}}_{m,\mathbf{q}} = \frac{\Lambda^{\boldsymbol{\delta}}_m}{2} \left(1 + e^{i\mathbf{q}\cdot\boldsymbol{\delta}}\right) \ , \quad \Lambda^{\boldsymbol{\delta}}_m = \Lambda_m \left[1, -1^m, \lambda_m\right] \ , \quad \text{with} \quad m = 1, 2 \ , \tag{S12}$$

and $\lambda_m$ denotes a possible anisotropy between the $\boldsymbol{\delta}_{1,2}$ and $\boldsymbol{\delta}_3$ directions.

The phonon propagator reads

$$D^{mm'}_{\mathbf{q}\mathbf{q}'}(z) = \langle\langle \mathcal{B}_{m\mathbf{q}}; \mathcal{B}^\dagger_{m'\mathbf{q}'} \rangle\rangle(z) \ , \tag{S13}$$

where $z = \omega + i0^+$. In the absence of scattering from Majorana fermions, the free propagator is diagonal, both, in momentum $\mathbf{q}$ and mode index $m$,

$$\left[D^{mm'}_{\mathbf{q}\mathbf{q}'}(z)\right]_0 = \delta_{\mathbf{q}\mathbf{q}'}\delta_{mm'}D^0_{m\mathbf{q}}(z), \quad \text{with,} \quad D^0_{m\mathbf{q}}(z) = \frac{1}{z-\omega_{m\mathbf{q}}} - \frac{1}{z+\omega_{m\mathbf{q}}} = \frac{2\omega_{m\mathbf{q}}}{z^2-\omega^2_{m\mathbf{q}}} . \tag{S14}$$

The phonon propagator in the interacting system can be evaluated via Dyson's equation

$$D^{mm'}_{\mathbf{q}}(z) = \left[\left[D^0_{m\mathbf{q}}(z)\right]^{-1} - \Sigma^{mm'}_{\mathbf{q}}(z)\right]^{-1}, \quad \text{with,} \quad \Sigma^{mm'}_{\mathbf{q}}(z) = \langle\langle \mathcal{H}_{m\mathbf{q}}; \mathcal{H}^\dagger_{m'\mathbf{q}}\rangle\rangle(z) . \tag{S15}$$

In principle the self-energy $\Sigma^{mm'}_{\mathbf{q}}$ is not diagonal in the polarization indeces $m$, leading to a phonon mixing upon inversion of the right hand side of the Dyson equation, i.e.

$$D^{mm}_{\mathbf{q}}(z) \neq D^m_{\mathbf{q}}(z), \quad \text{with,} \quad D^m_{\mathbf{q}}(z) = \left[\left[D^0_{m\mathbf{q}}(z)\right]^{-1} - \Sigma^{mm}_{\mathbf{q}}(z)\right]^{-1} \tag{S16}$$

To incorporate the magnetic field and the momentum into the results for the uniform gauge sector $\eta_{\boldsymbol{\delta}} = 1$, the analytical calculations are adapted accordingly. Hamiltonian (S9) can again be diagonalized by Fourier transformation with $c_{\mathbf{k}} = \frac{1}{\sqrt{2N}}\sum_{\mathbf{r}} e^{-i\mathbf{k}\cdot\mathbf{r}}c_{\mathbf{r}}$, with $\{c_{\mathbf{k}}, c^\dagger_{\mathbf{k}'}\} = \delta_{\mathbf{k},\mathbf{k}'}$, and similarly for the $c'$ operators, where $\mathbf{k} = (k_1 + \frac{\pi}{L})\mathbf{G}_1 + (k_2 + \frac{\pi}{L})\mathbf{G}_2$, $k_j = 2\pi l_j/L$, $\mathbf{G}_1 = \frac{1}{3a}(\sqrt{3}\boldsymbol{e}_x - \boldsymbol{e}_y)$, and $\mathbf{G}_2 = \frac{2}{3a}\boldsymbol{e}_y$. The Hamiltonian in reciprocal space reads

$$H_K = \frac{1}{2}\sum_{\mathbf{k}} \Psi^\dagger_{\mathbf{k}} \begin{pmatrix} \epsilon_{\mathbf{k}} & 0 \\ 0 & -\epsilon_{\mathbf{k}} \end{pmatrix} \Psi_{\mathbf{k}}, \; \epsilon_{\mathbf{k}} = \sqrt{|t_{\mathbf{k}}|^2 + w^2_{\mathbf{k}}}, \quad \text{with,} \tag{S17}$$

$$t_{\mathbf{k}} = \sum_{\boldsymbol{\delta}} t_{\boldsymbol{\delta};\mathbf{k}}, \quad t_{\boldsymbol{\delta};\mathbf{k}} = -\frac{i}{2}J_{\boldsymbol{\delta}}e^{-i\mathbf{k}\cdot\boldsymbol{\delta}}, \quad \text{and} \quad w_{\mathbf{k}} = \frac{\tilde{J}}{2}\sum_{j=1}^{3}(-)^j \sin(\mathbf{k}\cdot\mathbf{a}_j) .$$

The spinor $\Psi^\dagger_{\mathbf{k}} = (d^\dagger_{1,\mathbf{k}}, d^\dagger_{2,\mathbf{k}})$ comprises the two quasiparticle bands. $h_{\boldsymbol{\delta};\mathbf{q}}$ from Eq. (S11) is

$$h_{\boldsymbol{\delta};\mathbf{q}} = \frac{1}{2\sqrt{N}}\sum_{\mathbf{k}} \Psi^\dagger_{\mathbf{k}-\mathbf{q}}\tilde{V}_{\boldsymbol{\delta};\mathbf{k}-\mathbf{q},\mathbf{k}}\Psi_{\mathbf{k}} , \quad \text{with,} \tag{S18}$$

$$\tilde{V}^{\mu\nu}_{\boldsymbol{\delta};\mathbf{k}_1,\mathbf{k}_2} = \frac{-1}{4\sqrt{\epsilon_{\mathbf{k}_1}\epsilon_{\mathbf{k}_2}}}\left[t^*_{\boldsymbol{\delta};\mathbf{k}_1}t_{\mathbf{k}_2}\xi^{\mu\nu}_{\mathbf{k}_1\mathbf{k}_2} + t^*_{\mathbf{k}_1}t_{\boldsymbol{\delta};\mathbf{k}_2}\xi^{\nu\mu}_{\mathbf{k}_2\mathbf{k}_1}\right], \quad \text{and} \quad \xi^{\mu\nu}_{\mathbf{k}_1\mathbf{k}_2} = (-1)^\nu\sqrt{\frac{\epsilon_{\mathbf{k}_1} + (-1)^\mu w_{\mathbf{k}_1}}{\epsilon_{\mathbf{k}_2} + (-1)^\nu w_{\mathbf{k}_2}}} ,$$

where the indeces take the values $\mu, \nu = 1, 2$. The diagonal matrix elements of $\tilde{V}$ refer to particle-hole (ph), and the off-diagonal to particle-particle (pp) scattering processes. The former contribute with a relative plus sign in $\tilde{V}$ while the latter with a minus one. Complex conjugation results in $\tilde{V}^{\mu\nu *}_{\boldsymbol{\delta};\mathbf{k}_1,\mathbf{k}_2} = \tilde{V}^{\nu\mu}_{\boldsymbol{\delta};\mathbf{k}_2,\mathbf{k}_1}$, leading to $h^\dagger_{\boldsymbol{\delta};\mathbf{q}} = h_{\boldsymbol{\delta};-\mathbf{q}}$, which ensures the hermiticity of $H_K$ and $H_{KP}$. A straightforward evaluation, using (S11), (S13), (S18), and [S9] yields

$$\Sigma^{mm'}_{\mathbf{q}}(z) = \frac{1}{N}\sum_{\mathbf{k}}\left[V^{\mu\mu}_{\mathbf{kq}m}V^{\mu\mu *}_{\mathbf{kq}m'}\mathcal{L}^{ph}_{\mathbf{k},\mathbf{q}}(z) - V^{\mu\bar{\mu}}_{\mathbf{kq}m}V^{\mu\bar{\mu}*}_{\mathbf{kq}m'}\mathcal{L}^{pp}_{\mathbf{k},\mathbf{q}}(z)\right], \quad \text{with,} \tag{S19}$$

$$\mathcal{L}^{ph}_{\mathbf{k},\mathbf{q}}(z) = \sum_{\pm}\frac{f_{\mathbf{k}+\mathbf{q}} - f_{\mathbf{k}}}{\epsilon_{\mathbf{k}+\mathbf{q}} - \epsilon_{\mathbf{k}} \mp z} , \quad \text{and} \quad \mathcal{L}^{pp}_{\mathbf{k},\mathbf{q}}(z) = \sum_{\pm}\frac{1 - f_{\mathbf{k}+\mathbf{q}} - f_{\mathbf{k}}}{\epsilon_{\mathbf{k}+\mathbf{q}} + \epsilon_{\mathbf{k}} \mp z} .$$

The scattering amplitude for both contributions is a real number, determined by the matrix $V_{\mathbf{kq}m} = \sum_{\boldsymbol{\delta}}\Lambda^{\boldsymbol{\delta}}_{\mathbf{q}m}\tilde{V}_{\boldsymbol{\delta};\mathbf{k}+\mathbf{q},\mathbf{k}}$, while $\mu(\bar{\mu})$ can be chosen either $\mu = 1(2)$ or $\mu = 2(1)$. The particle-hole $\mathcal{L}^{ph}_{ij}(z)$, and particle-particle $\mathcal{L}^{pp}_{ij}(z)$ Lindhard functions set the frequency and temperature dependence, with $f_j$ being the Fermi-Dirac distribution $f_j = 1/(e^{\epsilon_j/T}+1)$. For $q = 0$, $\mathcal{L}^{ph}_{\mathbf{k},\mathbf{0}}(z)$ is identically zero and only the pp-channel contributes to the self-energy. After some algebra one arrives in Eq. (5) of the manuscript. For $\mathbf{q} \neq 0$ the self-energy cannot be expressed in terms of a single function only.

In Fig. S2(a), we present results for the effect of the magnetic field on the self-energy $\Sigma(\omega)$ at $\mathbf{q} \neq 0$. Various values of the NNN coupling $\tilde{J}$ are depicted. This figure clearly demonstrates that the magnetic field is relevant only for low frequencies due to the gap-opening. This can be important for acoustic phonons [S10], however, for the optical phonon modes beyond the gap, magnetic fields play no role.

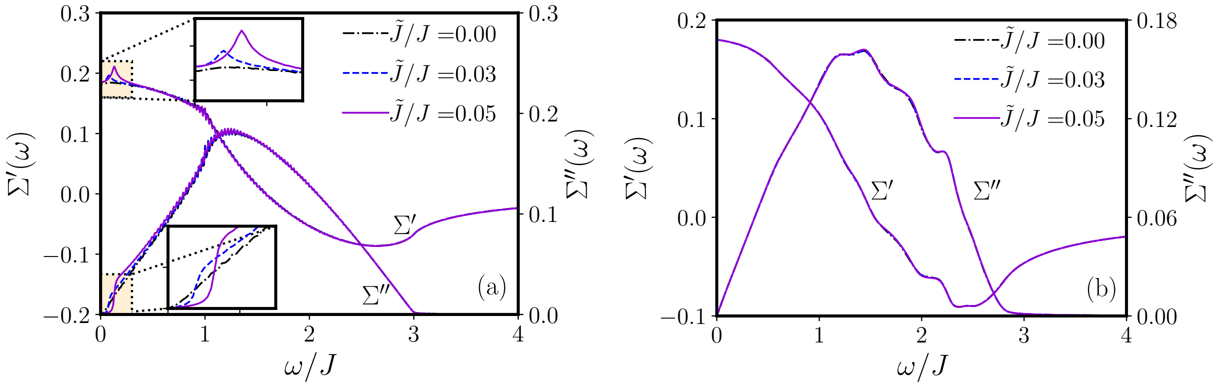


FIG. S2. Phonon self-energy $\Sigma(\omega)$ for various NNN couplings $\tilde{J}/J = 0, 0.03, 0.05$. (a) Within the uniform gauge sector at $T/J = 0.01$ and for $L = 200$. (b) For random gauges, averaging over $N_R = 200$ maximally disordered sectors at $T/J = 0.3$ and $L = 30$.

## III. NUMERICAL METHOD FOR DISORDERED GAUGE SECTORS

For temperatures $T \gg T^*$, gauge excitations need to be taken into account. For that, a random averaging over maximally disordered configurations is sufficient to describe the fermionic system's properties [S11]. Since translation invariance is broken, we resort to numerical methods in real space, while following the same steps as for the analytical calculation. This means, we first set a real space spinor with the $2N$ Majorana operators, $C^\dagger = (c_{\mathbf{r}_1}, \ldots, c_{\mathbf{r}_N}, c'_{\mathbf{r}_1-\boldsymbol{\delta}_3}, \ldots, c'_{\mathbf{r}_N-\boldsymbol{\delta}_3})$ as the original representation to set up operators, $\hat{O} = C^\dagger O C$. Next, we change into a Dirac fermion basis $D = FC$ where $D^\dagger = (d^\dagger_{\mathbf{k}_1}, \ldots, d^\dagger_{\mathbf{k}_N}, d_{\mathbf{k}_1}, \ldots, d_{\mathbf{k}_N})$ and $F$ is the Fourier transform with its matrix elements being defined as $F_{ij} = e^{i\mathbf{k}_i\cdot\mathbf{R}_j}/\sqrt{2N}$ with $\mathbf{R}_j = \mathbf{r}_j$ or $\mathbf{R}_j = \mathbf{r}_j - \boldsymbol{\delta}_3$ for $1 \le j \le N$ or $N+1 \le j \le 2N$, respectively. The last step, is to switch into the Hamiltonian's diagonal basis, $E^\dagger = (e^\dagger_1, \ldots, e^\dagger_N, e_1, \ldots, e_N)$, with $E = UD$, where $U$ is a numerical Bogoliubov transformation. The self-energy from Eq. (S15) is then evaluated by writing operators as

$$\hat{O} = E^\dagger \tilde{O} E, \quad \text{with} \quad \tilde{O} = U^\dagger[(2F^\dagger)O(2F)]U \;, \tag{S20}$$

resulting in an expression similar to Eq. (S19), i.e.,

$$\Sigma^{mm'}_{\mathbf{q}}(z) = 2\sum_{i,j=1}^{N}\Big[(\tilde{\mathcal{H}}_{m\mathbf{q}})_{\bar{i}\bar{j}}\Big[(\tilde{\mathcal{H}}^\dagger_{m'\mathbf{q}})_{\bar{j}\bar{i}} - (\tilde{\mathcal{H}}^\dagger_{m'\mathbf{q}})_{ij}\Big]\mathcal{L}^{ph}_{ij}(z) + (\tilde{\mathcal{H}}_{m\mathbf{q}})_{i\bar{j}}\Big[(\tilde{\mathcal{H}}^\dagger_{m'\mathbf{q}})_{\bar{j}i} + (\tilde{\mathcal{H}}^\dagger_{m'\mathbf{q}})_{i\bar{j}}\Big]\mathcal{L}^{pp}_{ij}(z)\Big] \tag{S21}$$

where $\bar{i}(\bar{j}) = i + N(j+N)$, $\tilde{\mathcal{H}}$ is dictated by Eqs. (S11) and (S20), while the Lindhard functions are given by

$$\mathcal{L}^{ph}_{ij}(z) = \sum_{\pm}\frac{f_i - f_j}{\epsilon_i - \epsilon_j \mp z} \;, \qquad \mathcal{L}^{pp}_{ij}(z) = \sum_{\pm}\frac{1 - f_i - f_j}{\epsilon_i + \epsilon_j \mp z} \;, \tag{S22}$$

with $\epsilon_i$ the energy eigenvalues and $f_i$ the corresponding Fermi-Dirac distribution.

In Fig. S2(b), we present numerical results for $\Sigma(\omega)$ obtained numerically after random averaging over $N_R = 200$ maximally disordered sectors on a system with a linear dimension $L = 30$ and at $T = 0.3J$. Fig. S2(b) illustrates that elevated temperatures completely conceal the weak effect of the magnetic field, in the whole frequency range.

## IV. RAMAN CROSS SECTION

Here we explain the steps which lead to the Eq. (6) of the main text for the Raman intensities. First we consider the Raman cross section of a ficticious system at momentum zero and energy $z$, comprising two optical phonons,

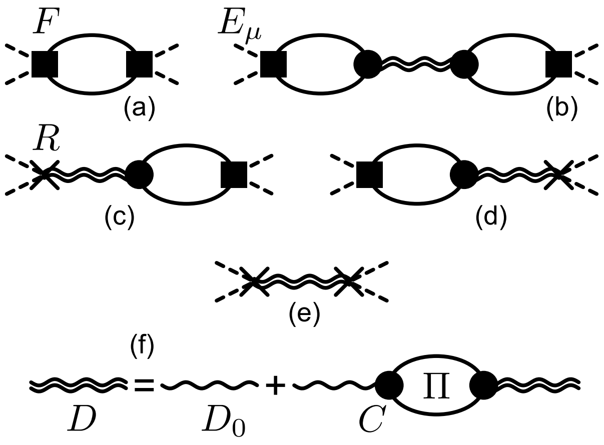


FIG. S3. (a)-(e) Diagrams contributing to the Raman cross section Eq. (S24). Dashed line: photons. $E_\mu$: electric field. Solid square $F$, cross $R$, and solid circle $C$: Raman and fermion-phonon vertices. Solid steady line: fermions with ellipse $\Pi$ particle-hole Greens function. (f) Dyson equation Eq. (S25) for single (double) wiggly line: bare (dressed) phonon Greens function, $\mathbb{D}_0(\mathbb{D})$.

with *bare* Greens functions $D_{0i=1,2}(z)$, coupled to a fermionic background, with a particle-hole Greens function $\Pi(z)$. Both phonons and the fermionic background are assumed to be Raman active. We proceed by strongly simplifying all Raman operators $F$ and $R_{i=1,2}$ of the fermionic background and the phonons, as well as the fermion-phonon coupling matrix elements $C_{i=1,2}$ to be real *constants*. The total cross section $-\mathrm{Im}[I(\omega+i0^+)]$ derives from a trace over the Dyson equation (apart from the trivial fluctuation-dissipation prefactor)

$$\begin{aligned} I(z) &= \begin{bmatrix} F \\ R_1 \\ R_2 \end{bmatrix}^\dagger \left[\mathbb{G}_0^{-1}(z) - \mathbb{V}\right]^{-1} \begin{bmatrix} F \\ R_1 \\ R_2 \end{bmatrix} \\ \mathbb{G}_0(z) &= \begin{bmatrix} \Pi(z) & 0 & 0 \\ 0 & D_{01}(z) & 0 \\ 0 & 0 & D_{02}(z) \end{bmatrix} \\ \mathbb{V} &= \begin{bmatrix} 0 & C_1 & C_2 \\ C_1 & 0 & 0 \\ C_2 & 0 & 0 \end{bmatrix} . \end{aligned} \tag{S23}$$

This can be written differently

$$I_n(z)=\Pi(z)+\begin{bmatrix} r_1+\Pi(z)C_1 \\ r_2+\Pi(z)C_2 \end{bmatrix}^T \mathbb{D}(z) \begin{bmatrix} r_1+C_1\Pi(z) \\ r_2+C_2\Pi(z) \end{bmatrix}, \tag{S24}$$

where $\mathbb{D}(z)$ is the *dressed* $2\times 2$ phonon Greens function

$$\mathbb{D}(z) = \left[\mathbb{D}_0^{-1}(z) - \begin{bmatrix} C_1^2 & C_1C_2 \\ C_1C_2 & C_2^2 \end{bmatrix} \Pi(z)\right]^{-1}, \tag{S25}$$

with $\mathbb{D}_0(z)$ being the lower $2\times 2$ block of $\mathbb{G}_0(z)$ and henceforth we normalize $r_i = R_i/F$, and $I_n(z) = I(z)/F^2$. Eq. (S24) can either be derived by simple algebra from Eq. (S23), or it can be visualized by iterating the corresponding diagrams. The latter is shown in Fig. S3.

Several comments regarding Eq. (S24) are in order. First, contributions of type $\Pi(z)C_i\mathbb{D}_{ij}(z)r_j$, Figs. S3(c) and S3(d), from the second addend on its right-hand side represent interference effects between the phononic and the fermionic Raman scattering, i.e., the *Fano effect.* Second, the Fano effect is intrinsically tied to the renormalization of the bare phonon by the fermions. Speaking differently, for any $C_{1,2}\neq 0$ and for a finite fermionic and phononic Raman vertex $r_{1,2}^{-1}\neq 0$, the Fano effect is unavoidable. Third, for the problem formulated, the Fano effect is always *complete.* I.e. irrespective of the particular form of $\Pi(z)$ and the parameters $C_{1,2}$ and $r_{1,2}$, each phonon gives rise to one energy at which the cross section is *strictly zero.* Fourth, and as a direct consequence of the latter, the causality

of the cross section is delicate. E.g., simplifying $\mathbb{D}(z)$ in Eq. (S25) by discarding the off-diagonal self-energy, in order to decouple the two phonons, will inevitably lead to regimes of parameters $C_{1,2}$, for which the cross section turns *negative* over certain ranges of $\omega$. This has to be kept in mind when performing additional simplifications.

Turning to the coupled phonon-Majorana system of the present work, evaluating the diagrams of Fig. S3 from first principles is infeasible. This is, because it involves momentum summations over form-factors contained in $F$ *and* $R_i$. While the former is known from [S12–S14], the latter is unknown and may differ between the two optical phonons considered here. In addition to that the amplitudes of $F$ and $R_i$ are modulated by the scattering geometry. In this situation, and to make progress, we perform four *phenomenological* simplifications. (i) We remain with mere constants for $F$ and $R_i$. These will differ for different scattering geometries. (ii) The constants $C_{1,2}$, displayed in Eq. (S24) are used as free parameters, independent of $\mathbb{D}(z)$, in order to adjust the magnitude of the Fano effect. (iii) We assume $\mathbb{D}(z)$ to be diagonal. (iv) Most important, since the spectrum of the purely magnetic Raman cross section of Refs. [S12–S14] is very similar in shape to the spectrum of the normalized part of phonon self-energy $-\mathrm{Im}\Sigma(\omega + i0^+)$, we approximate $\Pi(z) \approx \Sigma(z)[J/(\Lambda_1\Lambda_2)]^2$ on the right-hand side of Eq. (S23). Altogether one obtains

$$I_n(z) \approx \Pi(z) + \sum_{i=1,2} [r_i + C_i \Pi(z)]^2 \mathbb{D}_{ii}(z)\,, \tag{S26}$$

which is Eq. (6) of the main text, upon replacing $\mathbb{D}_{ii}(z)$ with $D_{mm}(z)$.


* a.metavitsiadis@tu-bs.de
† w.natori@imperial.ac.uk
‡ j.knolle@tum.de
§ w.brenig@tu-bs.de



[S1] G. Jackeli and G. Khaliullin, Phys. Rev. Lett. **102**, 017205 (2009).
[S2] J. G. Rau, E. K.-H. Lee, and H.-Y. Kee, Phys. Rev. Lett. **112**, 077204 (2014).
[S3] K. I. Kugel and D. I. Khomskii, Sov. Phys. Usp. **25**, 231 (1982).
[S4] G. Khaliullin, Prog. Theor. Phys. Suppl. **160**, 155 (2005).
[S5] S. M. Winter, A. A. Tsirlin, M. Daghofer, J. van den Brink, Y. Singh, P. Gegenwart, and R. Valentí, J. Phys.: Condens. Matter **29**, 493002 (2017).
[S6] W. M. H. Natori, R. Moessner, and J. Knolle, Phys. Rev. B **100**, 144403 (2019).
[S7] A. Kitaev, Annals of Physics **321**, 2 (2006), january Special Issue.
[S8] Y.-Z. You, I. Kimchi, and A. Vishwanath, Phys. Rev. B **86**, 085145 (2012).
[S9] To arrive at the analytical expression for the self energy we have also used the useful properties for $\tilde{V}$, $\tilde{V}^{\mu\nu}_{\mathbf{k}_1,\mathbf{k}_2} = -\tilde{V}^{\bar{\mu}\bar{\nu}}_{\mathbf{k}_1,\mathbf{k}_2}$ with $\bar{\mu} = \mu - (-1)^\mu$ and $\tilde{V}^{\mu\nu}_{-\mathbf{k}_1,-\mathbf{k}_2} = -\tilde{V}^{\bar{\nu}\bar{\mu}}_{\mathbf{k}_2,\mathbf{k}_1}$, where we have dropped the $\boldsymbol{\delta}$ index for simplicity.
[S10] M. Ye, R. M. Fernandes, and N. B. Perkins, Phys. Rev. Research **2**, 033180 (2020).
[S11] A. Metavitsiadis, A. Pidatella, and W. Brenig, Phys. Rev. B **96**, 205121 (2017).
[S12] P. A. Fleury and R. Loudon, Phys. Rev. **166**, 514 (1968).
[S13] J. Nasu, J. Knolle, D. L. Kovrizhin, Y. Motome, and R. Moessner, Nature Physics **12**, 912 (2016).
[S14] J. Knolle, G.-W. Chern, D. L. Kovrizhin, R. Moessner, and N. B. Perkins, Phys. Rev. Lett. **113**, 187201 (2014).
